# Supplementary material for: Modeling the Data-Generating Process is Necessary for Out-of-Distribution Generalization
Source: arXiv:2206.07837 source file (2024-05-17)
Supplement: Supplementary file 1 [file rebuttal_expts.tex]

\section{\new{Evaluation on additional baselines}}
\label{app:rebuttal_expts}
% We perform additional experiments based on reviewer suggestions.

% \subsection{Evaluation on additional baselines}

\newjuhclhcz{\new{We evaluate all three datasets -- Synthetic, MNIST and small NORB on information bottleneck
based invariant risk minimization (IB-IRM) and information bottleneck based empirical risk minimization (IB-ERM) (Ahuja et al., 2021).These two methods have been recently proposed for out-of-distribution generalization; they combine the information bottleneck constraint with invariance constraint.  %demonstrate its effectiveness for 

We add these new results (marked in blue) to  Tables \ref{table:results_synthetic_ib}, \ref{table:results_mnist_ib}, \ref{table:results_norb_ib}. We observe that IB-IRM performs comparable to other baselines on synthetic and small NORB datasets (in fact, worse than ERM on multi-attribute shift in small NORB). While IB-IRM outperforms other baselines on multi-attribute shift in MNIST, our method performs better than both IB-ERM and IB-IRM in all datasets. The results demonstrate that even in comparison to these newer methods, \cacm achieves superior performance across datasets and shifts.
 
\textbf{References}\footnote{Added here to avoid changing citation numbers for ease in referencing. We will update the references in the final version.}\\\\
Ahuja, K., Caballero, E., Zhang, D., Bengio, Y., Mitliagkas, I., \& Rish, I. (2021). Invariance Principle Meets Information Bottleneck for Out-of-Distribution Generalization. \textit{NeurIPS}.}}


\begin{comment}
\subsection{\selected shift}

\selected shifts arise due to selection effect in the data generating process and induce an association between $Y$ and $\asel$. \todo{this may be a problematic example...if larger hospitals have more diseased, then there is already a confounding wrt A. Let's avoid giving examples--I suggest moving this to D.2 so that it is at the same place as confounded. And use the same blue font to denote new text. } A data point is included in the sample only if selection variable $S=1$ holds; $S$ is a function of $Y$ and $\asel$.
The selection criterion may differ between domains~\citep{veitch2021counterfactual}.

In Proposition~\ref{thm:ind-constraints}, we see that for the \selected shift, $\vecX_c \perp\!\!\perp \asel|Y$; $\vecX_c \not\!\perp\!\!\!\perp \asel$ (also, $\vecX_c \perp\!\!\perp \asel|Y, E$; $\vecX_c \not\!\perp\!\!\!\perp \asel|E$) whereas for the \confounded shift, $\vecX_c \perp\!\!\perp \aconf$; $\vecX_c \not\!\perp\!\!\!\perp \aconf|Y$ (also, $\vecX_c \perp\!\!\perp \aconf|E$; $\vecX_c \not\!\perp\!\!\!\perp \aconf|Y, E$). We construct our \selected setup similar to Synthetic \causal (Section~\ref{app:datasets}) and \confounded setups (Section~\ref{app:sec_causal_confounded}) to demonstrate the importance of using the valid independence constraints for different kinds of shifts.

We have three environments, $E_1, E_2 \in \mathcal{E}_{tr}$ (training) and $E_3 \in \mathcal{E}_{te}$ (test). $\vecX_c$ has a uniform distribution $\mathrm{Uniform}[0, 1]$ across all environments. Our selection variable $s$ is a function of $Y$ and $\asel$ and our observed input $\vecX$ is 2-dimensional and formed by concatenating $\vecX_c$ and $\asel$. We add 10\% noise to $Y$ in all environments.


\begin{align*}
    \vecX_c \in \mathrm{Uniform}[0, 1];
    \quad \quad \asel \in \{1, 2, 3, 4\}
\end{align*}

\begin{align*}
    y_{true} = \left\{ \begin{array}{lll}
0 & \mbox{if $\vecX_c \in [0, 0.25)$ }
&  \\ 
1 & \mbox{if $\vecX_c \in [0.25, 0.5)$ }
%\mathrm{Uniform}[0.25, 0.5) & \mbox{if y = 1}
&  \\
2 & \mbox{if $\vecX_c \in [0.5, 0.75)$ }
%\mathrm{Uniform}[0.4, 0.6) & \mbox{if y = 2}
&  \\
3 & \mbox{if $\vecX_c \in [0.75, 1.0]$ }
%\mathrm{Uniform}[0.6, 0.8) & \mbox{if y = 3}
&  \\
\end{array}\right.
\end{align*}


\begin{align*}
    s = 1 \quad if\left\{ \begin{array}{rcl}
\asel + y = 4 & \mbox{with prob. =}
& p \\ \asel - y = 1 & \mbox{with prob. =} & 1-p
\end{array}\right.
    \quad ; p_{E_1} = 0.9, p_{E_2} = 1.0, p_{E_3} = 0.0
\end{align*}

\begin{table}[h]
\caption{Comparison of  constraints $\vecX_c \perp\!\!\perp \vecA|Y, E$ and $\vecX_c \perp\!\!\perp \vecA|E$ in \selected and \confounded shifts. $\vecX_c \perp\!\!\perp \vecA|Y, E$ is a correct constraint for \selected shift but invalid for \confounded shift; $\vecX_c \perp\!\!\perp \vecA|E$ is a correct constraint for \confounded shift but invalid for \selected shift.}
  \medskip
  \label{table:app_results_selected}
  \centering
  \small
  \begin{tabular}{lcc}
    \toprule
    \multirow{2}{*}{\textbf{Constraint}} & \multicolumn{2}{c}{\textbf{Accuracy}}\\
        \cmidrule(r){2-3}
    & $\asel$ & $\aconf$ \\ \midrule
    $\vecX_c \perp\!\!\perp \vecA|E$ & 72.3 $\pm$ 0.9 & \textbf{62.4 $\pm$ 1.9}\\
    $\vecX_c \perp\!\!\perp \vecA|Y, E$ & \textbf{88.7 $\pm$ 0.9} & 56.0 $\pm$ 1.0\\ 
    \bottomrule
  \end{tabular}
\end{table}
  
Table~\ref{table:app_results_selected} compares the performance of the constraints discussed above in synthetic \selected and \confounded setups. We can see that the valid constraints derived from the graph significantly outperform the incorrect constraints in both shifts, consistent with our findings in Section~\ref{app:sec_causal_confounded}. Hence, the information on the specific relationship between $Y$ and $\vecA$ is necessary for obtaining an optimal predictor.
\end{comment}
